# Supplementary material for: Robust Relationship Between Mid-latitudes CAPE and Moist Static Energy in Present and Future Simulations
Source: arXiv:2212.05548 source file (2022-12-13)
Supplement: Supplementary file 1 [file CAPE_future_SI.pdf]

# Supporting Information for "Robust Relationship Between Mid-latitudes CAPE and Moist Static Energy in Present and Future Simulations"

Ziwei Wang[1,2] and Elisabeth J. Moyer[1,2]

[1]Department of the Geophysical Sciences, University of Chicago, Chicago, Illinois
[2]Center for Robust Decision-making on Climate and Energy Policy (RDCEP), University of Chicago, Chicago, Illinois

December 3, 2022

## Contents

**S1 Observational studies of CAPE** **2**

**S2 Data sampling and model validation** **2**

**S3 Methods - subsetting and averaging** **3**

**S4 Theories and simple models** **4**
- S4.1 Zero-buoyancy model (SO13) . . . . . 4
- S4.2 EB96 and AE17 models . . . . . 5

**S5 Supporting material for Results** **6**
- S5.1 Main text Figure 1 . . . . . 6
- S5.2 Main text Figure 2 . . . . . 8
- S5.3 Main text Figure 3 . . . . . 10
- S5.4 Main text Figure 4 . . . . . 14

**S6 Alternative versions of synthetics** **16**
- S6.1 SO13 compared to itself vs. to CTRL . . . . . 16
- S6.2 Effect of fixed versus adjusted RH on synthetic transformations . . . . . 16

**S7 Latitudinal dependence of changes** **17**

# S1 Observational studies of CAPE

This work documents CAPE sensitivity to warming in a high-resolution model. Multiple prior studies have examined CAPE changes in historical observational records. These studies are difficult to compare to, as they typically focus on decadal-scale trends in the tropics. Because secular temperature increases are relatively small (and are sometimes not specified), any interpretation of the results as predictive of long-term future changes should be made carefully.

Trends in historical studies are typically given in units of J/kg/decade. The model simulations we used involve pseudo-global warming inputs that should represent 100 years of warming; the average surface temperature increase in our domain is 4.65 K or ∼0.465 K/decade. Mean CAPE is 684 J/kg in present conditions and 1003 in simulated future warmer conditions. We expressed its rate of increase as 13%/K but could alternatively specify it as 32 J/kg/decade.

Gettelman et al. [2002] examined profiles from 15 tropical radiosonde stations, 10 of which had 40-year continuous records (1958-1997), and found that mean CAPE increased nearly 24% while temperature increased less than 0.5 degrees, i.e. a change of ∼40%/K or 85 J/kg/decade. In these data RH is fairly stable and the lapse rate reduces slightly. Other observational studies provide less complete information but show broadly similar rates of CAPE increase, e.g. 40 J/kg/decade over India from radiosondes [Murugavel et al., 2012], or over 100 J/kg/decade in the tropics in ERA40 reanalysis [Riemann-Campe et al., 2009]. Interpretation of these results is difficult but Gettelman et al. [2002] does provide complete information on surface conditions and their observed fractional change in CAPE is larger than simple theories would support.

# S2 Data sampling and model validation

To facilitate comparing model output to observations, we use throughout this work the same spatial sampling in this analysis as in the observational study of Wang et al. [2021], which selected 80 U.S. radiosonde stations. When analyzing model output, we use the 80 grid cells that most closely match these locations (Figure S2a).

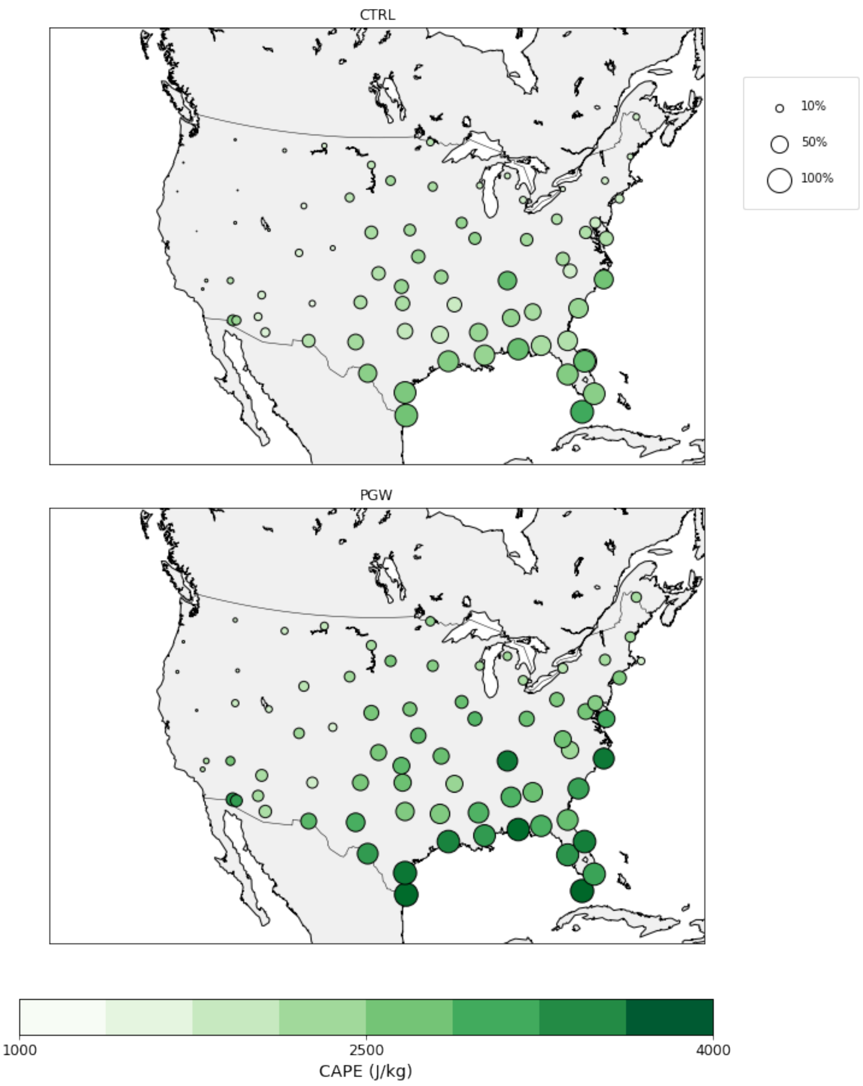


Figure S2a: Locations of the 80 grid cells used in this analysis, matching the IGRA weather stations of Wang et al. [2021]. Stations sample diverse conditions with strong gradients of mean CAPE in latitude and longitude. Symbol areas denote the fraction of summer (MJJA) samples that are above 1000 J/kg in CTRL (top) and PGW (bottom) model runs, and color denotes the mean CAPE of those samples > 1000 J/kg. Most extreme CAPE observations are from Southeast stations near the Gulf coast.

Although Wang et al. [2021] extensively compared the model CTRL run with radiosonde data, we extend the comparison here using figures developed for this study. As shown in Figure S2b, the CAPE-MSE relationships between radiosonde and the model used are broadly similar. While mean summertime CAPE values are similar at 680 and 686 J/kg in observations and model CTRL, respectively, the WRF model slightly underestimates the extreme high tail of CAPE by 6–10%, as noted by Wang et al. [2021], and also produces too-low values in low-CAPE conditions (< 50th percentile, or < 43 J/kg in CTRL). Overall, however, the model matches observations reasonably well for conditions with CAPE > 1000 J/kg (the 73rd quantile in CTRL). Both datasets show a similar proportion of profiles with zero CAPE (36% in observations, vs. 40% in CTRL and 36% in PGW runs).

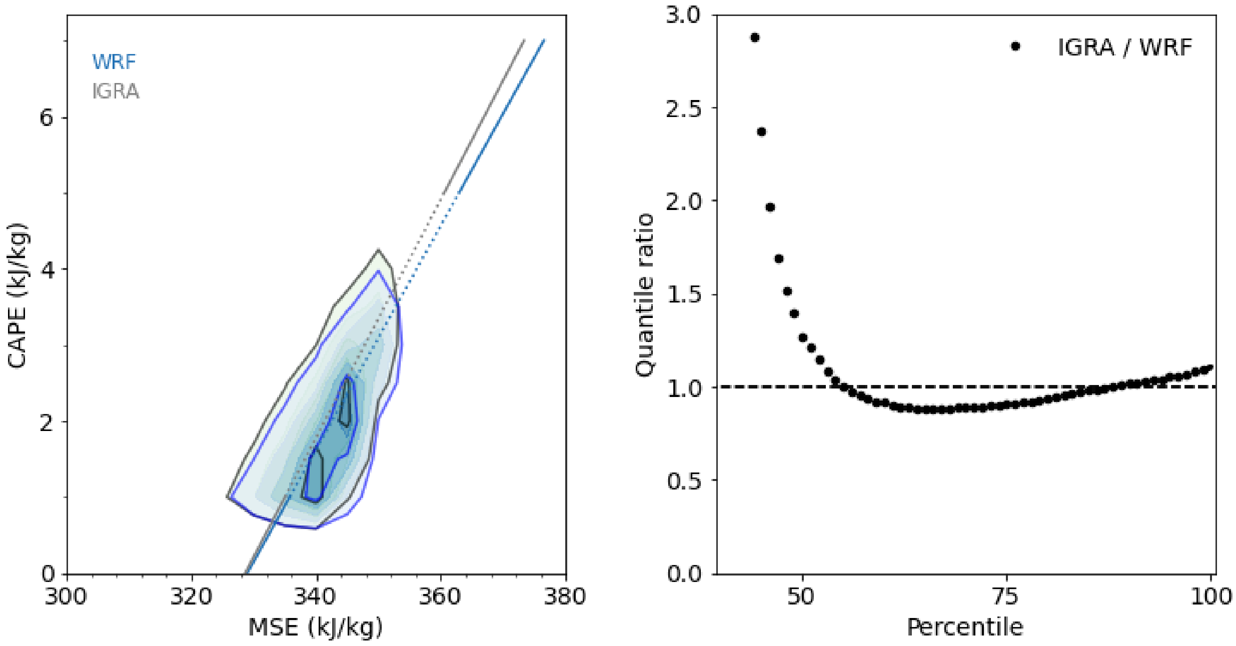


Figure S2b: Comparison of the WRF CTRL run against observations (IGRA), as (left) CAPE-MSE density plot and (right) quantile ratio. For WRF and IGRA, respectively, the variances explained are 65% and 66%, slopes are 0.147 and 0.157, and x-intercepts are 329.0 and 328.6 kJ/kg. Note that the regressions are fitted with all cases with CAPE >1000 J/kg without binning.

## S3 Methods - subsetting and averaging

In this paper, we generally subset the full dataset to focus on high CAPE conditions. In the CTRL model run, 27% of profiles have CAPE > 1000 J/kg, i.e. values exceeding this threshold occur above the 73rd percentile. We subset the data in two ways.

1) We generally apply a *fractional cut*, i.e. we subset to CAPE or MSE above a given quantile (e.g., the 73rd percentile). This procedure produces the same number of samples in each case studied (e.g. CTRL and PGW climates), avoiding sampling biases that can be introduced by cutting at an absolute threshold.

2) In one case we apply an *absolute cut*, subsetting to profiles with CAPE above a given absolute threshold value of ≥1000 J/kg. We apply this procedure primarily when evaluating the dependence between CAPE and MSE (main text Figure 3). In this case we are fitting CAPE-MSE relationships, so the absolute cut will not lead to an artificial bias, and it is important instead that the samples being compared cover analogous physical conditions. An addition case is Figure S5i, where we subset to high CAPE profiles using absolute cut.

When computing average climate parameters for the purpose of describing present-future changes, we typically use subsetted data. That is, the average change reported is the change in high-CAPE conditions. To construct our synthetic profiles, we estimate changes using a fractional cut at the 73rd percentile of CAPE. In this case, between CTRL and PGW the temperature increases by 3.92 K at the surface and 4.94 K at 200 hPa, and surface RH reduces by −0.92%. We use the full dataset when computing a temperature rise as a metric of climatological change, because the goal is to describe a general climate change rather than a change in only high CAPE conditions. In this case, between CTRL and PGW the temperature increases by 4.65 K at the surface and 4.05 K at 200 hPa. That is, future temperatures increases in low-CAPE conditions are stronger at the surface and weaker aloft than in high-CAPE conditions, in part because spatial differences: low-CAPE conditions are more prevalent at higher latitudes, where surface warming is stronger.

One additional complication arises for surface temperature because of the fact that stations have different elevations, and surface temperature is a strong function of elevation. If two subsets contain different sets of stations and therefore different distributions of elevation, their surface temperatures may differ simply because of station sampling and not because of a secular change at individual stations. The effect is small for the CTRL-PGW (present-future) comparison:

if station sampling is frozen at those of the CTRL 73rd percentile cut, the future temperature change is 3.91 K, vs. 3.92 K when allowing different station sampling.

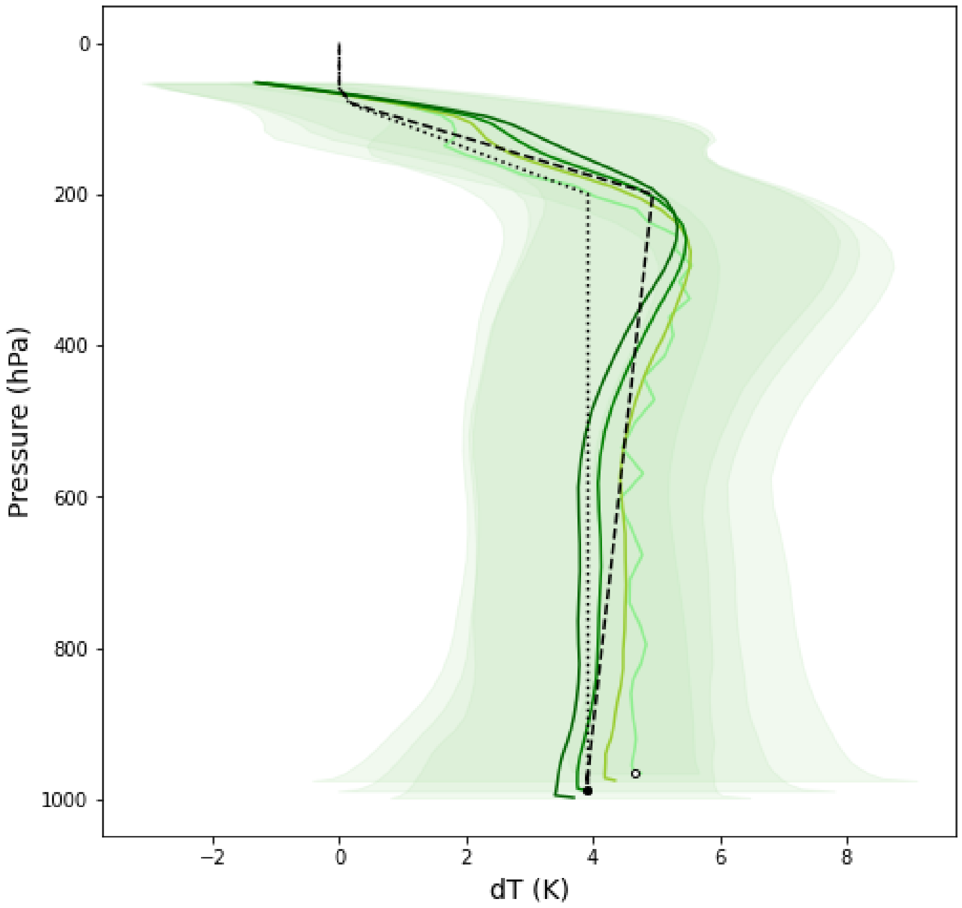


Figure S3a: Profile of temperature difference between CTRL and PGW model runs (green lines and shading), and assumptions for the lapse rate adj. (dashed line) and constant offset (dotted line) cases. Lines show mean values for four subdivisions of the data by quantiles of CAPE: all data (faintest) and $>$ 53th, 73th, and 95th (darkest) quantiles, chosen to approximate 100, 1000 , and 3000 J/kg in CTRL. (Actual quantile values are 89, 991, and 2989 J/kg.) Shading shows the envelope for 25th–75th percentiles of each subset. In general, in the lower latitudes where CAPE values are high, surface warming is weakest and the surface pressure is lowest. We use the 73rd quantile ($\sim$1000 J/kg CTRL CAPE) as our benchmark in this analysis, yielding a surface temperature change of 3.92 K (dot); for comparison we also show the all-data mean surface temperature change of 4.65 K (circle). Note that this all-data mean surface is at higher altitude and lower pressure than are the high-CAPE subsets.

# S4 Theories and simple models

In this study we test how well several theories or simple models reproduce present-day mid-latitudes CAPE distributions and their future changes. This section provides further details and describes how these theories are applied to our datasets to generate predicted ‘conversion rates’ of MSE surplus to CAPE.

## S4.1 Zero-buoyancy model (SO13)

The zero-buoyancy model of atmospheric profiles in a convective environment is first described in Singh and O’Gorman [2013] (hereafter, SO13). The model derives environmental profiles from the assumption of neutrality and a specified entrainment rate. It has been shown to capture the fundamental physics of CAPE (or buoyancy) dependence on changing sea surface temperature and RH [Seeley and Romps, 2015]. However, since the model is designed to represent mean conditions in convection-dominated regimes, it is may not capture mid-latitudes CAPE distributions well.

The SO13 model requires four inputs – surface temperature, surface specific humidity (used to derive the moist adiabat), environmental relative humidity (assumed to be constant across all levels), and the level of neutral buoyancy (LNB) – plus the choice of one free parameter, the entrainment rate $\varepsilon$. For surface quantities, we use model 2-meter temperature and associated specific humidities. We use an environmental RH of 0.44, the mean from levels below 200 hPa in PGW (future) summer profiles. (In CTRL the mean RH is similar, 0.43.) Note that Singh and O’Gorman [2013] did not calculate the LNB in each profile but instead assumed it occurred where $T = 200$ K. This assumption may be acceptable in their study with profiles governed by RCE, but it does not allow for zero CAPE unless the environmental profiles is saturated. For our midlatitudes dataset, where 40% of profiles have zero CAPE even in the convective summertime; the realistic LNB height are included as input to ensure the SO13 captures the percent of zero incidences.

Finally, we derive an entrainment rate by fitting to match the mean CAPE above 1000 J/kg and find that the appropriate rate is $\varepsilon$=0.62 in PGW and 0.60 in CTRL; we use 0.62.

## S4.2 EB96 and AE17 models

The EB96 framework [Emanuel and Bister, 1996] assumes the whole atmosphere can be treated as one "heat engine", that redistributes energy between the surface level (where heat is added) and the emission level (where heat is emitted through radiative cooling) [Klein, 1997]. Its mathematical formulation is:

$$CAPE \approx (h_s - h_m)\left(1 - \frac{\overline{T}}{T_s}\right) \quad (1)$$

Here $h_s$ and $h_m$ are the MSE at surface and mid-troposphere, respectively, if multiplied by a mass flux their difference would equal a net heat flux. The second term is analogous to a Carnot efficiency: $T_s$ is surface temperature and $\overline{T}$ is the temperature at which radiation is emitted to space. EB96 could therefore be interpreted as representing the maximum possible conversion rate of a heat flux to kinetic energy.

Previous authors [Romps, 2008] have suggested that EB96 should overestimate the conversion rate of moist static energy deficit to CAPE, pointing out that the input of energy from latent heat does not occur only at the warmest temperatures, near the top of boundary layer, as is required for Carnot efficiency in the heat engine model if latent heat is considered the input. However, Pauluis and Held [2002] note that a more appropriate thermodynamic analogy is to a steam cycle, which can achieve Carnot. Romps [2008] also note factors that would limit the conversion of CAPE to kinetic energy, including frictional dissipation of falling condensates and high levels of entrainment, but those factors would not contribute to the relationship between MSE and CAPE.

The AE17 model [Agard and Emanuel, 2017] describes CAPE as being proportional to the surplus of boundary layer MSE compared to the free troposphere dry static energy ($D_o$). Assuming that the $h_m$ and $D_o$ are close enough since the moisture availability is limited at 650 hPa, AE17 could be rewritten as:

$$CAPE \approx (h_s - h_m) \cdot \ln\left(T_h / T_{LNB}\right) \quad (2)$$

where $T_h$ is the boundary layer temperature, and $T_{LNB}$ is the temperature at the level of neutral buoyancy. Surface and boundary layer temperatures are similar ($T_h \approx T_s$), but because the level of neutral buoyancy typically lies well above the mean level of emission to space ($T_{LNB} < \overline{T}$), the term representing the conversion rate of MSE surplus to CAPE will therefore be larger in AE17 than in EB96.

We derive theoretical conversion rates for the two models above by aggregating all profiles with CAPE exceeding 1000 J/kg into a single mean temperature profile, instead of considering atmospheric profiles separately. The 1000 J/kg cutoff ensures that this mean profile is not dominated by atmospheric conditions that produce zero CAPE. This approach differs from that used by Li and Chavas [2021], who predict the conversion rate for AE17 by considering individual profiles.

For AE17, we determine the level of neutral buoyancy in the mean profile, and approximate the top of the boundary layer as the location of the level of free convection. For EB96, we take the surface temperature of the mean profile. To derive $\overline{T}$, we do not derive a radiative cooling profile from the mean temperature profile, but use that of EB96 Experiment I, which is designed to correspond to conditions where CAPE can accumulate to a large magnitude. As described in EB96, $\overline{T}$ is then calculated by taking the inverse of the inverse temperature weighted by the radiative cooling rate. (The radiative cooling rate sums both longwave and shortwave contributions.) The process of calculating theoretical conversion rates is identical for both model and observed profiles, but note that the radionsone dataset has substantial missing data, so contains only a subset (56%) of the sampling in model output. Tables S4a and S4b below show the relevant pressures, temperatures, and coefficients derived from model runs and observations, as well as the empirical slope of the CAPE-$h_s - h_m$ relationship in each dataset.

| | $z_{LFC}$ | $T_h$ | $z_{LNB}$ | $T_{LNB}$ | coefficient | emp. slope |
|---|---|---|---|---|---|---|
| CTRL | 0.3 km | 292 K | 14 km | 211 K | 0.32 | 0.17 |
| PGW | 0.3 km | 294 K | 15 km | 210 K | 0.34 | 0.18 |

Table S4a: AE17: parameters derived from mean summertime profiles, predicted conversion rates, and empirical CAPE-MSE surplus slope in two model runs (CTRL and PGW). The LFC ($z_{LFC}$) is assumed to approximate the top of the boundary layer ($T_h$).

|  | $T_s$ | $z_e$ | $T_e$ | coefficient | emp. slope |
|---|---|---|---|---|---|
| CTRL | 302 K | 8.8 km | 248 K | 0.18 | 0.17 |
| PGW | 305 K | 9.1 km | 252 K | 0.18 | 0.18 |
| IGRA | 299 K | 9.1 km | 246 K | 0.18 | 0.18 |

Table S4b: EB96: parameters derived from mean summertime profiles, predicted conversion rates, and empirical CAPE-$h_s - h_m^*$ slopes in two model runs (CTRL, PGW) and observations (IGRA).

# S5 Supporting material for Results

## S5.1 Main text Figure 1

To assist in understanding the quantile ratio plot of manuscript Figure 1, we show the original CAPE distribution in current (CTRL) and future (PGW) climates in Figure S5a. The future distribution of CAPE broadens, less so than in a simple multiplicative shift of the distribution, as shown by the downward slope of the quantile ratio plot. Even so, the incidence of very large CAPE increases dramatically (Figure S5a, right).

The heat map of manuscript Figure 1 is also useful for visualizing synthetic distributions of future CAPE. Figure S5b shows analogous heatmaps for the *constant offset* and *SO13* synthetics. Regressions clearly show that CAPE changes are too large in *constant offset* and too small in *SO13*.

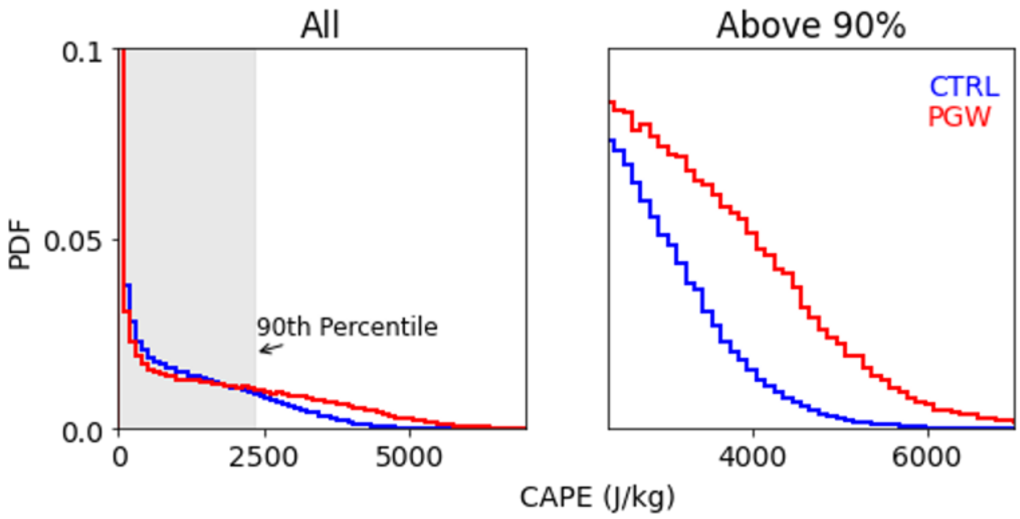


Figure S5a: Probability density functions of model CAPE in current (CTRL, blue) and future (PGW, red) climates show that the future distribution broadens, though less so than expected for a simple multiplicative shift. Right panel highlights quantiles above 90%. The y-axis on the left panel is truncated; zeroes make up nearly 40% of both datasets. The future climate (PGW) shows strongly increased incidences of extreme CAPE, with 24.3% incidence for CAPE > 2000 J/kg, compared to 13.5% incidence in CTRL.

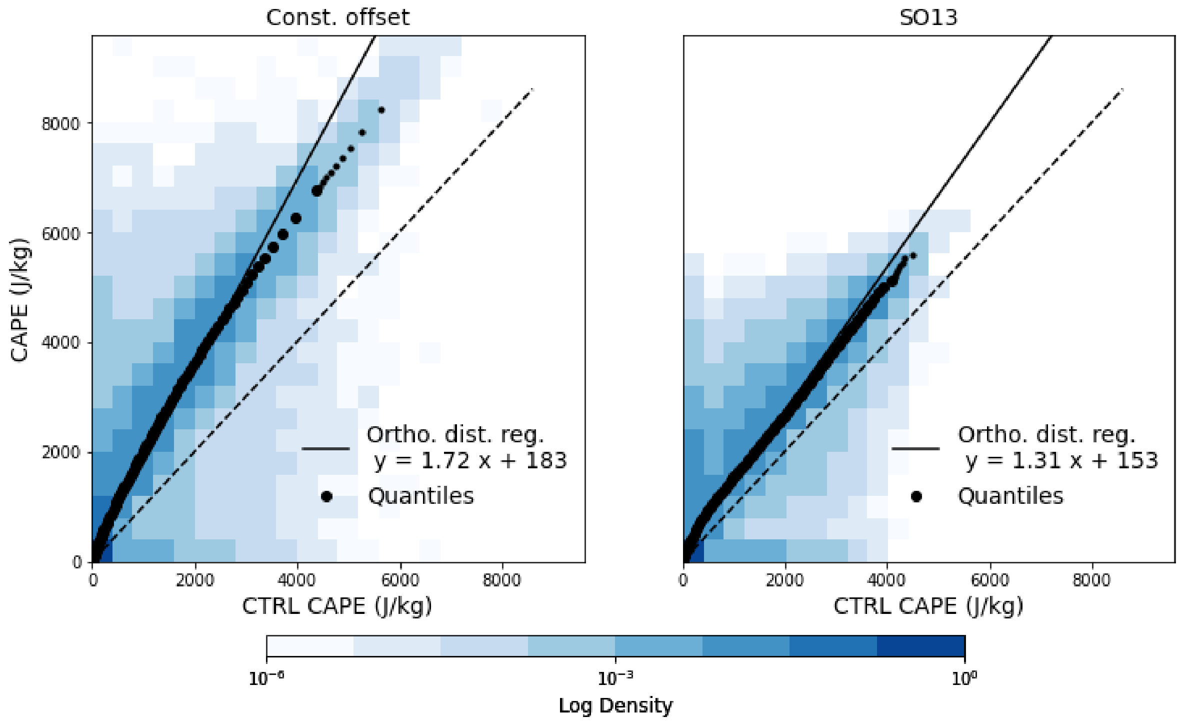


Figure S5b: As in main text Figure 1 left panel, but for (left) *constant-offset* and (right) *SO13*, calculated as described in text. CAPE changes are too large in *constant offset* and too small in *SO13*: dividing by 4.65 K produces fractional changes of 12%/K and 6%/K, respectively, vs. the 8%/K derived from model output. The quantiles of *SO13* lie close to the regression line since the zero-buoyancy model is designed for climatological mean conditions. For *constant offset* in particular, the quantiles fall below the orthogonal distance regression line above the 80th percentile. In both cases, however, the quantile regression matches the orthogonal distance regression reasonably well.

Because the *SO13* theory was developed to represent the *mean* profile in a highly convective environment, we also test whether it can capture the present-future CAPE change of an averaged profile in a mid-latitudes simulation. Because most mid-latitudes profiles are non-convective (CAPE in the mean profile is 24 J/kg in our present-day simulation), we restrict the comparison to 00 UTC (late afternoon locally; CAPE in the mean profile is 447 J/kg). The underprediction of *SO13* is even more substantial, at 5.1%/K vs. 17.6%/K in model output (triangles in Figure 1, right).

| | CAPE (WRF) | CAPE (SO13) | Frac. Change (WRF) | Frac. Change (SO13) | $T_s$ | Entrainment rate (SO13) |
|---|---|---|---|---|---|---|
| All profiles | 24 | 1604 | 14 | 1.31 | 296 | 0.62 |
| > 73% CAPE | 2569 | 2028 | 1.48 | 1.30 | 302 | 0.62 |
| 00 UTC | 447 | 447 | 2.27 | 1.27 | 300 | 0.13 |

Table S5a: Comparison of CAPE and their changes across different ways to derive mean profiles in high-res model and SO13. Note that for the fractional change analysis, the results are not affected by the choice of entrainment rate, as long as the entrainment rate is assumed to be unchanged between climate states.

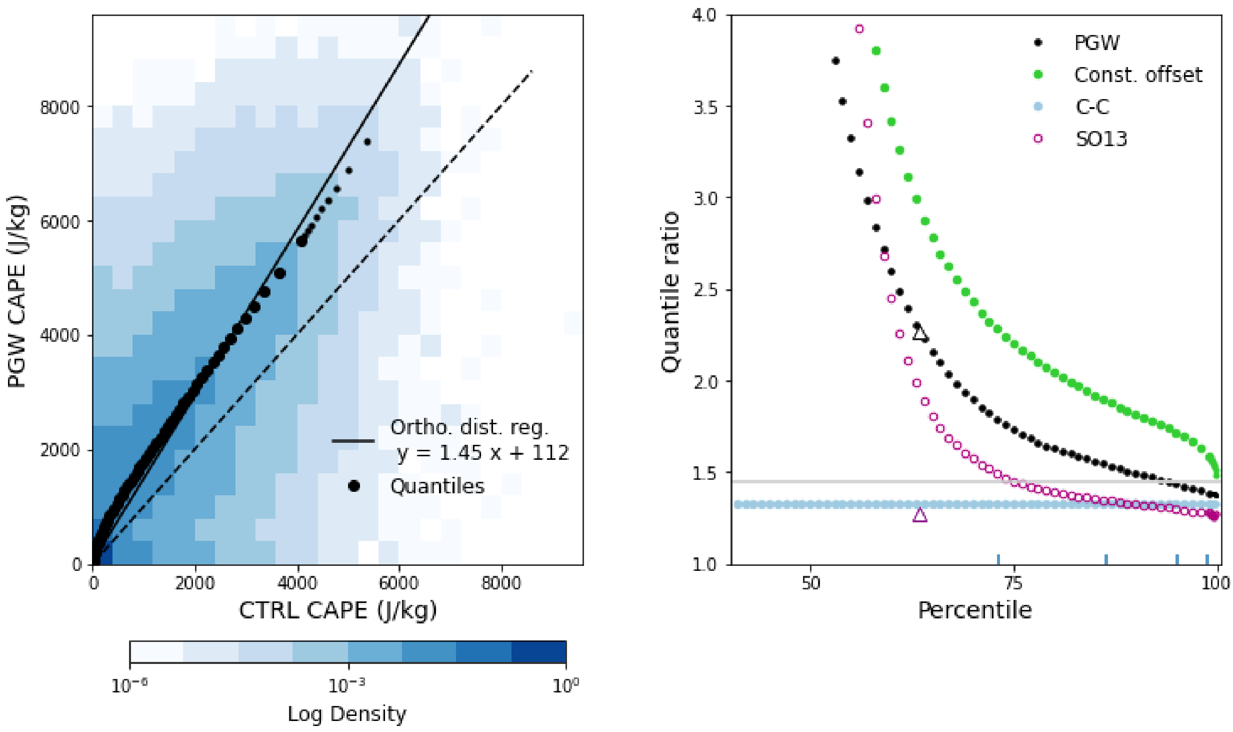


Figure S5c: (Left) Comparison of CAPE in present (CTRL) and future (PGW) model runs as a density plot of paired profiles. Dashed line is the one-to-one line; solid line is the orthogonal regression; and dots are quantiles of the distribution (large dots, Δ = 1% increments from 0-0.99; small dots Δ=0.1% above 0.99). (Right) Quantile ratio plot, comparing future/present CAPE quantiles from actual model output (black, dots as in L. panel), and three synthetic datasets: *C-C scaling* (light blue), *constant offset* (limegreen), and *SO13* (purple). For internal consistency, *SO13* changes are computed relative to its own CTRL distribution; see methods for details. Gray horizontal line marks the mean CAPE fractional change from the orthogonal distance regression line in left panel. Open triangles show the change in CAPE of the mean 00 UTC profile, for model output (black) and SO13 (purple). Their x-axis placement is at the quantile of the CTRL distribution that matches mean CTRL CAPE (447 J/kg). Four vertical tick bars mark the percentiles matching 1000, 2000, 3000, and 4000 J/kg (73.2%, 86.5%, 95.1%, and 98.9%, respectively). We begin the x-axis at 40% to omit quantiles where CTRL CAPE is zero. Model future CAPE changes resemble a constant offset with a small lapse rate adjustment.

## S5.2 Main text Figure 2

**Similarity of CAPE and MSE contours**

In all model runs, contours of CAPE in T,H space are closely aligned with those of moist static energy (MSE), suggesting a simple relationship (Figure S5d, left and center). However, that relationship shifts between present (CTRL) and future (PGW) runs: in the future simulation, a given CAPE value is associated with higher MSE (Figure S5d, right).

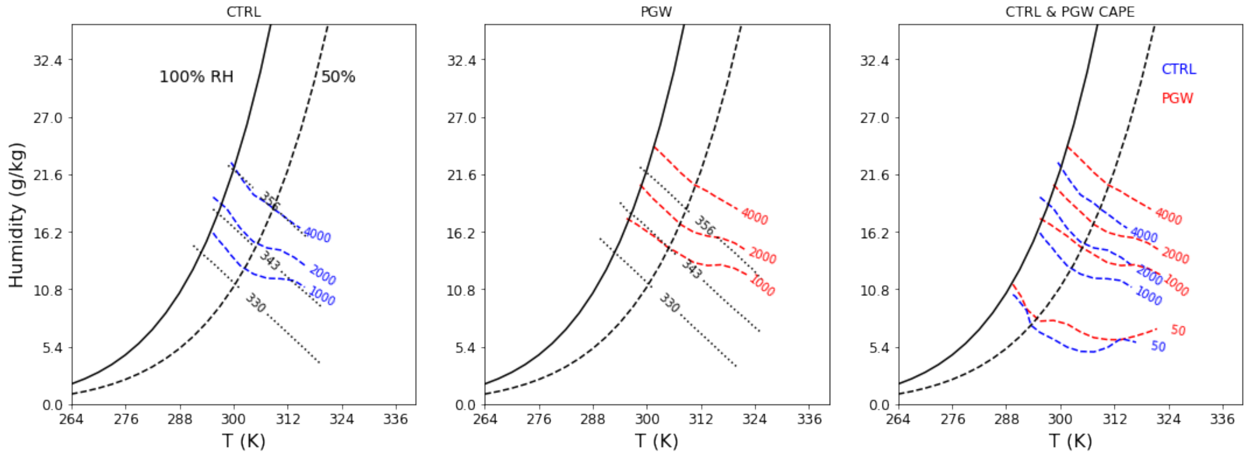


Figure S5d: Contours of CAPE and surface moist static energy (MSE) in model output for simulations in present (CTRL, left) and future (PGW, middle) conditions. CAPE contours follow those of moist static energy in the convection-promoting regime (CAPE > 1000 J/kg, RH > 40%), The relationship differs between CTRL and PGW (right). Contours here are cut off at RH=100%, as in main text Figure 2. Note that contours of CAPE become less aligned to those of surface MSE in conditions with low CAPE or very low surface relative humidity.

**Decomposition of sampling and environmental lapse rate effects**

We decompose the change in CAPE into a combination of *sampling effects* – increased sampling of hotter and wetter

surface conditions, and *lapse rate effects* – changes in environmental lapse rate for given T,H. It is the lapse rate effects that produce the shift in CAPE contours seen in Figure S5d. In general, future conditions produce “steeper” lapse rates, i.e. conditions further from the dry adiabat and therefore more stable to dry convection. We assume that the fractional changes due to sampling ($f_{samp}$) and environmental lapse rate ($f_{env}$) can be multiplied to derive total fractional change:

$$f_{total} = f_{samp} \times f_{env} \tag{3}$$

See Table S5b for confirmation that this assumption is reasonable in high-CAPE conditions.

We directly calculate $f_{env}$ as the averaged fractional difference across all bins in Figure S5e. We do not weight by the number of profiles per bin, but this choice has negligible effect on the value of $f_{env}$.

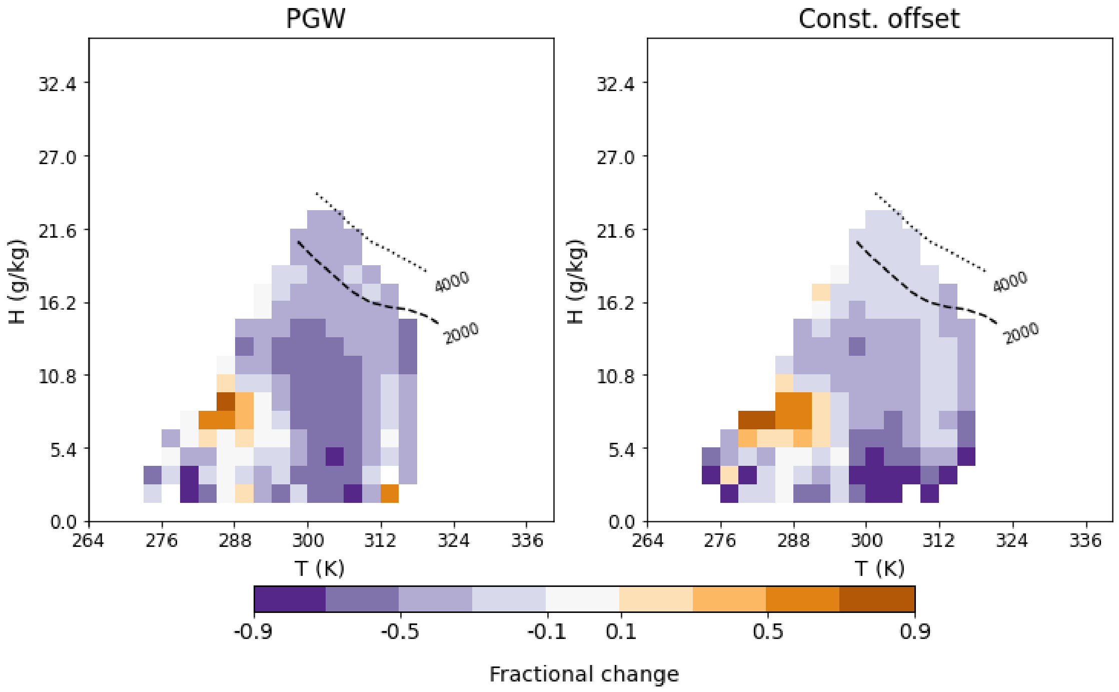


Figure S5e: Fractional changes in CAPE in T,H space in (left) PGW and (right) *constant offset* vs. CTRL, highlighting the effects of lapse rate changes. Even in *constant offset*, most bins show a damping of CAPE, since warmer bins now contain lapse rates originally characteristic of cooler temperatures. This damping effect is however stronger in actual model output. Bins that include less than 0.01% of the total number of profiles are removed.

Because the fractional change in CAPE is reasonably constant across T,H space (Figure S5e), the calculation of $f_{env}$ is generally unaffected by whether it is calculated with or without weighting by the number of profiles in each bin. The choice affects resulting values by no more than 2% in all but one case: for *constant offset* using all data, weighting by the number of profiles would produce a value higher by 14% (i.e. less damping by lapse rate changes).

To calculate $f_{samp}$, which is *only* the sampling effect, we consider how mean CAPE in the CTRL run would change if we used PGW sampling instead. That is, we construct an alternative mean CAPE for the CTRL dataset weighted by PGW sampling instead, and then take the ratio of this quantity to the actual mean CTRL CAPE: $f_{samp} = \overline{CAPE}_{PGW-samp}/\overline{CAPE}_{CTRL-true}$.

We show values of $f_{env}$, $f_{samp}$, and their product in Table S5b below, for various subsets of the data, and compare to the orthogonal regression slope. For the convective conditions studied in this work ($\geq$ 73rd quantile CAPE cutoff), the decomposition of model CAPE changes into $f_{env}$ and $f_{samp}$ factors matches the orthogonal regression slope reasonably well (1.37 vs. 1.41).

| Thresholds | | $f_{env}$ | $f_{samp}$ | $f_{env} \times f_{samp}$ | $f_{total}$ |
|---|---|---|---|---|---|
| ≥73% | PGW | 0.636 | 2.16 | 1.37 | 1.41 |
| | *constant offset* | *0.772* | *2.21* | *1.71* | *1.72* |
| ≥64.5% | PGW | 0.616 | 2.23 | 1.37 | 1.41 |
| | *constant offset* | *0.745* | *2.28* | *1.69* | *1.72* |
| ≥53.5% | PGW | 0.589 | 2.31 | 1.36 | 1.41 |
| | *constant offset* | *0.703* | *2.35* | *1.65* | *1.72* |
| ≥0% | PGW | 0.723 | 2.41 | 1.74 | 1.41 |
| | *constant offset* | *0.711* | *2.42* | *1.72* | *1.72* |

Table S5b: Derived fractional change in CAPE due to changes in the environmental lapse rate ($f_{env}$) and in sampling ($f_{samp}$), and the total change estimated as the product of the two effects ($f_{env} \times f_{samp}$). We show values for four subsets of the data, for CAPE above the 0th, 53.5th, 64.5th and 73rd percentiles. For comparison, last column shows the change estimated from the orthogonal distance regression slope using all data ($f_{total}$). Values are shown for both actual model output (PGW) and for the *constant offset* synthetic. If all data are used, predicted CAPE increases are large in both datasets. If restricted to convection-promoting conditions, the predicted increase in model CAPE becomes smaller, since lapse rate changes provide more damping (smaller $f_{env}$) and better agreement with the regression slope.

## S5.3 Main text Figure 3

**CAPE-MSE framework**

Figure S5f show how well could a model with MSE deficit ($h_d = h_s - h_m$, where $h_m$ is the minimum MSE in each profile) explain the variance in CAPE. Figures S5g–S5h test the robustness of CAPE-MSE framework when fitted on different subsets of data and when computed using different metrics. All three figures test for sensitivity to different latitudes, day-night contrast, seasonal cycle and year-to-year variability. Note that the regressions in SI are fitted with all cases with CAPE >1000 J/kg without binning, as opposed to the main text where we ensure homogenized sampling such that all CAPE bins are weighted the same.

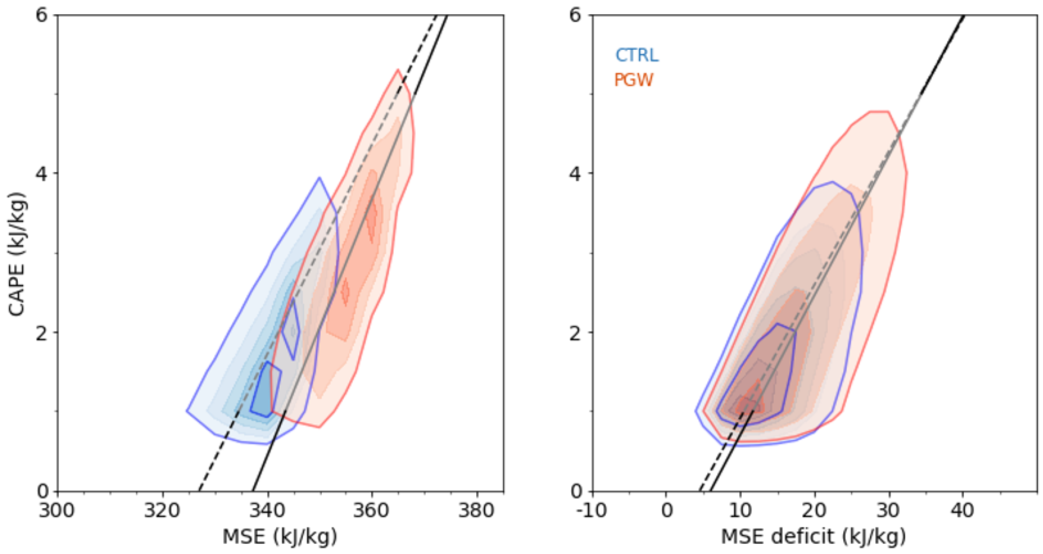


Figure S5f: Relationships between CAPE in N. America summertime and MSE (left) and $h_d$ (right), for CTRL (blue, dotted) and PGW (red, solid) runs. Color shading increments are 1.5% for the left panel and 0.75% for the right panel. Note that the full dataset is used to fit the orthogonal regression lines. Slopes of CAPE-MSE (left) are 0.132 and 0.161 for CTRL and PGW, respectively, and of CAPE-$h_d$ (right) are 0.168 and 0.176. X-intercepts for CAPE-MSE (left) are essentially equal to mid-tropospheric $\overline{h_m}$, at 327.0 and 337.3 kJ/kg for CTRL and PGW.

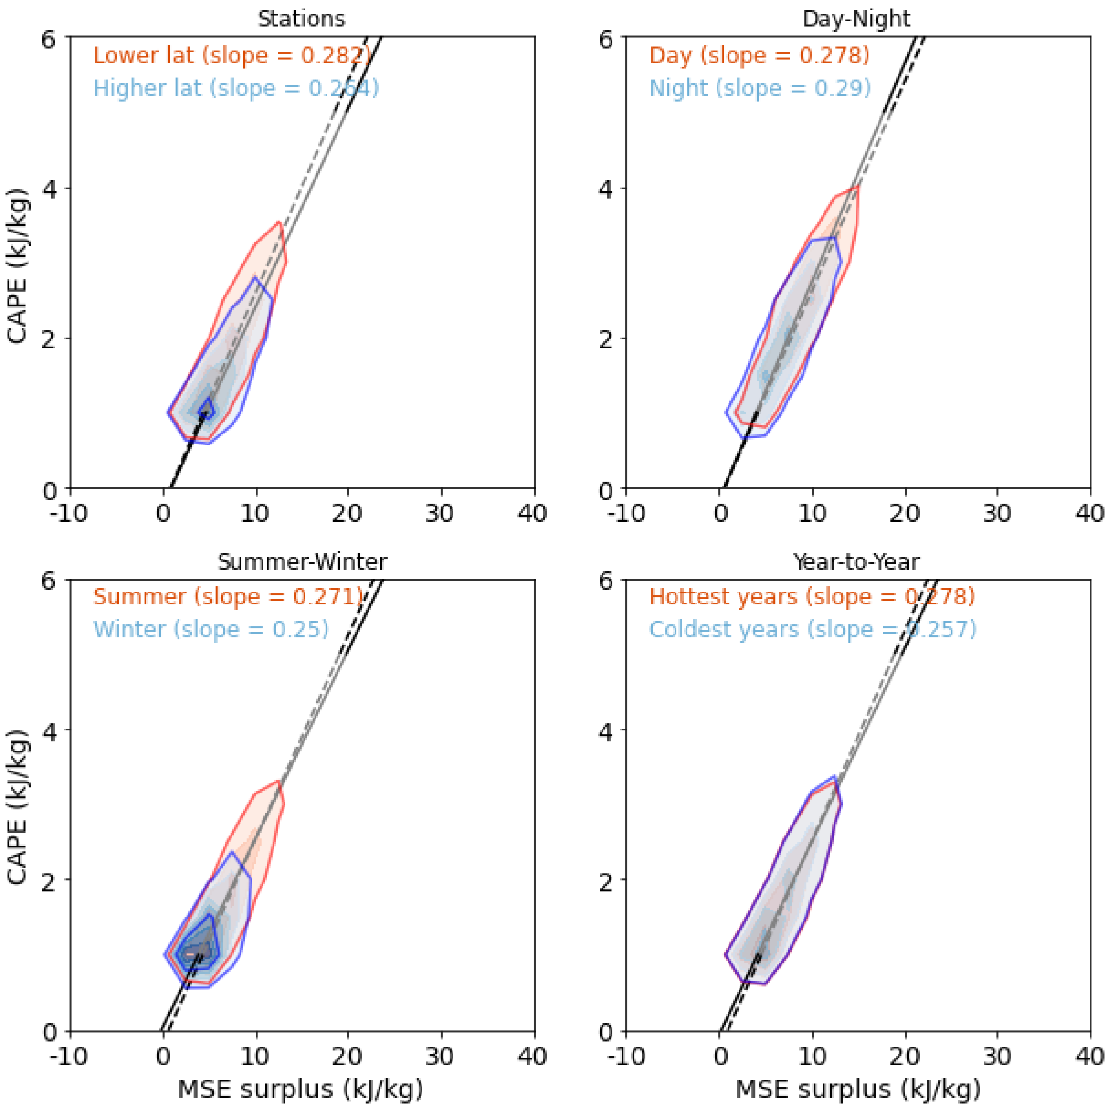


Figure S5g: Testing the robustness of the CAPE-saturation MSE surplus relationship with different subsets of the data. Figure uses only CAPE $\geq$ 1000 J/kg, and all besides lower left use summertime data only. MSE surplus are derived using the minimum saturation MSE in each individual profile. Each color shading is a 1.5% increment in density, and the orthogonal regression is fitted using binned median values. *Top left*: stations lower and higher latitude than 35N. *Top right*: daytime versus nighttime (using only stations below 30N, to avoid biasing the sampling). *Bottom left*: summertime (MJJA) versus wintertime (NDJF) (all other panels use summertime data only; note that the month of February 2005 in the PGW run is removed due to missing surface 2D fields). *Bottom right*: hottest 3 years (2001, 2006, 2012) versus coldest 3 years (2004, 2008, 2009). Intercepts and slopes are highly consistent across all conditions.

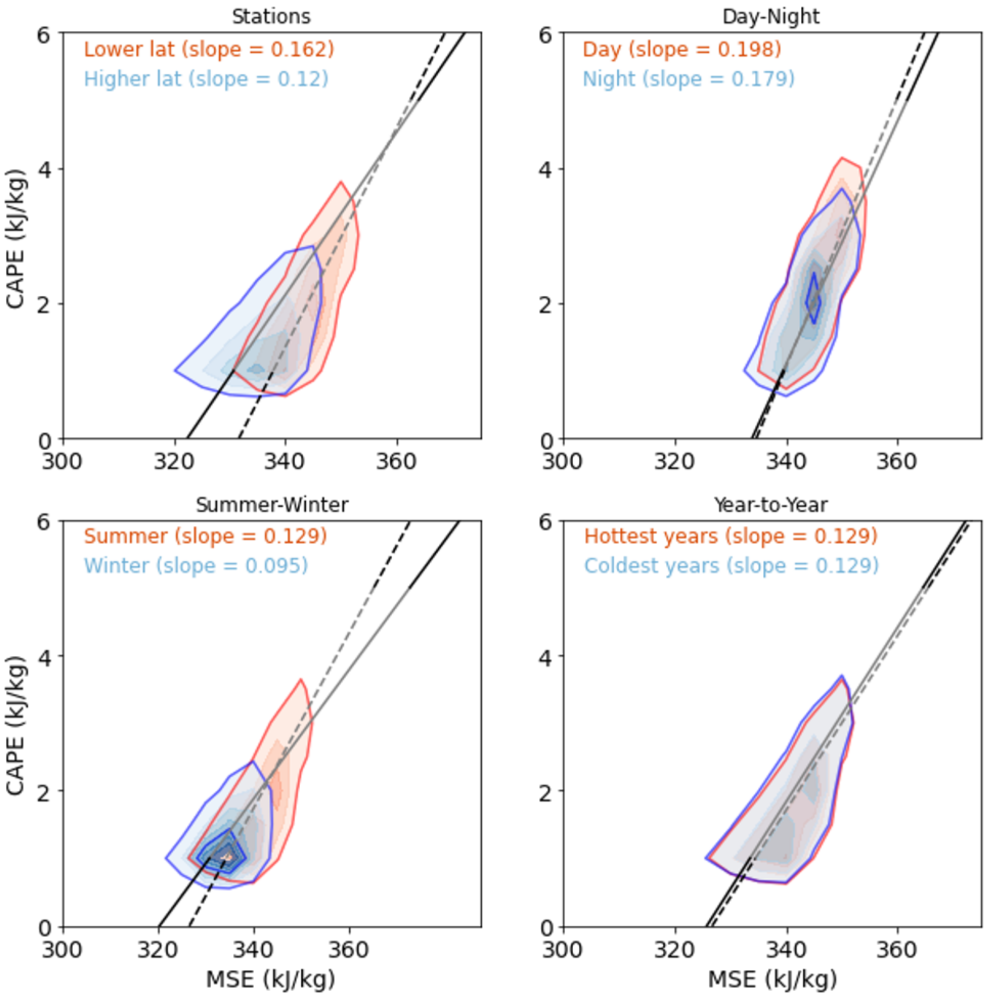


Figure S5h: As in Figure S5g, but now with MSE instead of MSE surplus on the x-axis. Color shading increment is 3%, and the orthogonal regression is fitted using binned median values. X-intercepts differ by latitude and by season because mid-tropospheric MSE is smaller at high vs. low latitudes or in winter vs. summer.

**Atmospheric profiles**

The atmospheric profiles are averaged across all conditions, and above high CAPE percentiles (73rd, 83.5th, and 95th), in order to highlight the sensitivity of temperature and MSE profiles to CAPE levels.

Figure S5i showed a subtle change in lapse rate in model output for future, warmer conditions, but a pronounced shift in MSE, with changes slightly larger in the mid-troposphere. Table S5c shows changes in temperature and MSE for all subsets of the data, and Table S5d decomposes changes in MSE (at surface, 650 hPa, and 200 hPa) into its relevant factors, for cases with CAPE $\geq$ 73rd percentile. In model output, the change in MSE at the surface is caused primarily by change in moisture (latent enthalpy), itself the result of higher temperature, though a reduction in RH moderates the result substantially. In the mid-troposphere, sensible and latent enthalpy make roughly equal contributions and the effects of small changes in RH are negligible, justifying our choice to neglect them in synthetics. The simple *lapse rate adjustment* synthetic captures MSE changes at surface and 650 mb reasonably well.

| Subsets | All cases | $\geq$53.5% | $\geq$73.0% | $\geq$98.9% |
|---|---|---|---|---|
| $\Delta T_s$ (K) | 4.65 | 4.3 | 3.92 | 3.95 |
| $\Delta T_{200}$ (K) | 3.98 | 4.55 | 4.94 | 5.02 |
| $\Delta MSE_s$ (kJ/kg) | 12.4 | 14.3 | 14.1 | 15.2 |
| $\Delta MSE_{650}$ (kJ/kg) | 8.3 | 8.1 | 7.6 | 6.9 |

Table S5c: Changes in temperature and MSE at surface and at altitude derived from the mean profiles of Figure S5i. All subsets of the data show increased MSE surplus in future (PGW) model output.

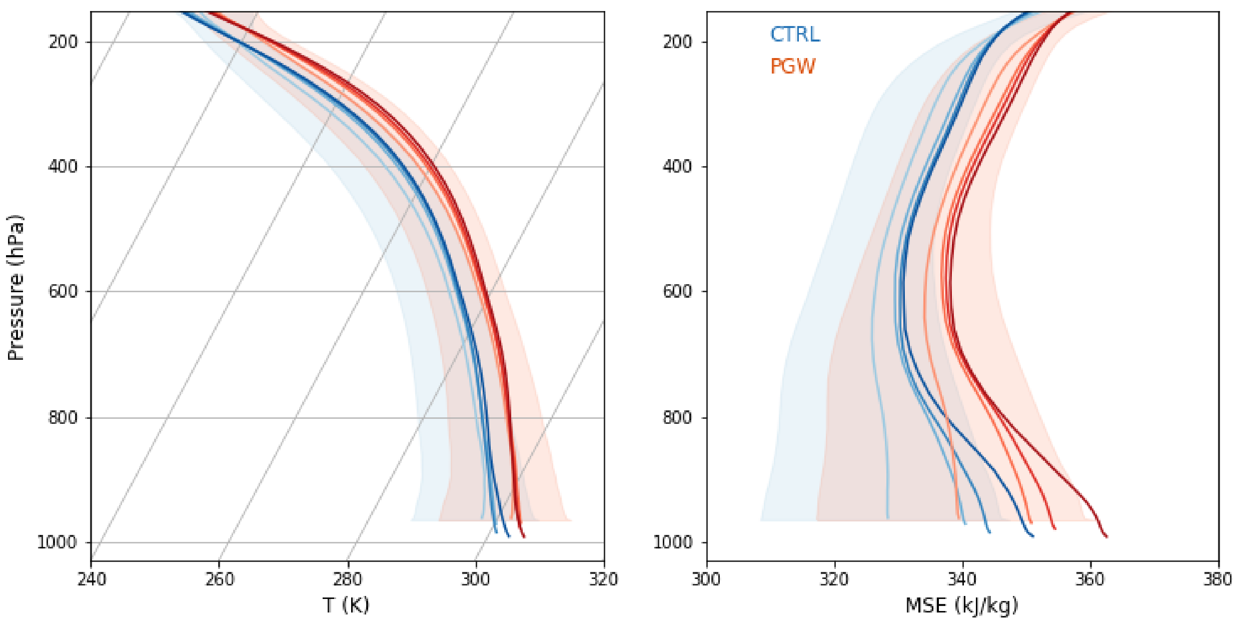


Figure S5i: Mean profiles of temperature (left) and moist static energy (right) in CTRL (blue) and PGW (red). Solid lines show mean profiles for four subsetting thresholds based on CAPE thresholds: from lightest to darkest, all cases and >100, 1000, and 4000 J/kg. Color shading marks envelope of 10th–90th percentiles of all cases. (Left): Lapse rate changes are weakly positive when subset to CAPE >1000 J/kg or higher. (Right): MSE gradients in lower troposphere are strongly related to CAPE and greater in high-CAPE subsets, while mean mid-tropospheric MSE ($\overline{h_m}$) shows little CAPE dependence. These results suggest that MSE profiles are highly informative of CAPE. Future $h_s$ increases more than $h_m$ because of nonlinear contribution of moisture. See Table S5c for values for $\Delta T_s$, $\Delta T_{200}$, $\overline{h_s}$, $\overline{h_m}$ of each subset, and fraction of $\Delta\overline{h_s}$ provided by latent heat.

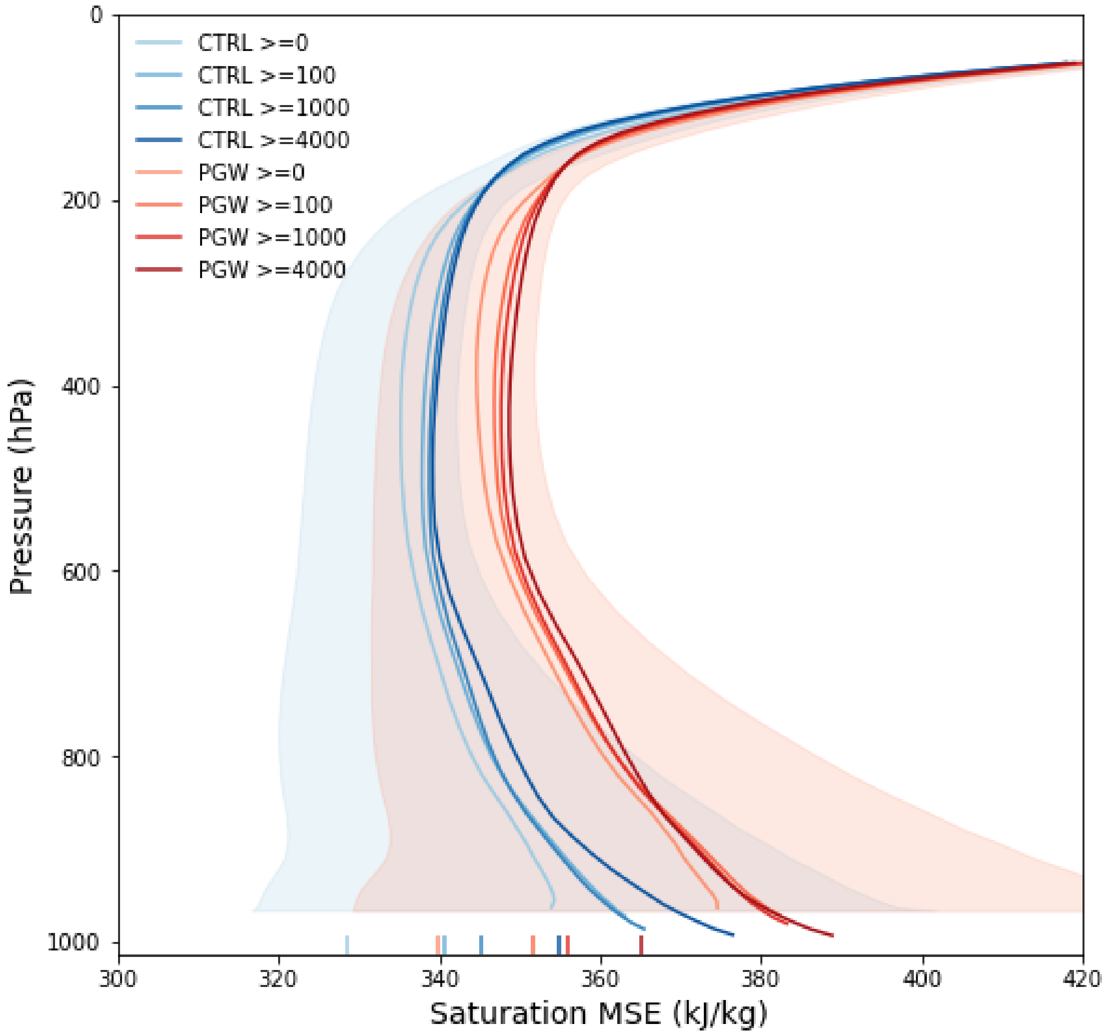


Figure S5j: As in Figure S5i, but showing profiles of saturation MSE instead of MSE. The subsetting and color coding conventions are the same as above. Surface MSE values of corresponding subset are marked with blue or red bars on x-axis.

| | | PGW change | Lapse rate adj. | Frac. Diff. (%) |
|---|---|---|---|---|
| Surface | Total MSE change | 14.1 | 12.6 | −10.6 |
| | Sensible enthalpy | 4.0 | 3.5 | −12.5 |
| | Latent enthalpy (RH effect only) | 10.1 (-0.6) | 9.1 (-0.3) | −9.9 |
| 650hPa | Total MSE change | 8.2 | 8.1 | −1.2 |
| | Sensible enthalpy | 4.1 | 4.4 | 7.3 |
| | Latent enthalpy (RH effect only) | 3.5 (-0.5) | 3.7 (-0.4) | 5.7 |
| | Geopotential | 0.6 | — | — |

Table S5d: Contributions to MSE changes from different factors, for both model output and *lapse rate adjustment*, using data $\geq$ 73rd percentile in CAPE. All values in units of kJ/kg and shown for the surface and for 650hPa, the level at which the MSE reaches a minimum. Decomposed terms are sensible enthalpy ($c_pT$), latent enthalpy ($L_vq$, with RH contribution in parentheses) and geopotential energy ($gz$). The simple *lapse rate adjustment* synthetic captures MSE changes reasonably well, so it is unsurprising that it best predicts future (PGW) CAPE distributional shift.

We can apply a single mean change in MSE surplus without imposing bias because for the high-CAPE conditions of interest, MSE surplus changes are uncorrelated with original values of either CAPE or MSE surplus (Figure S5k).

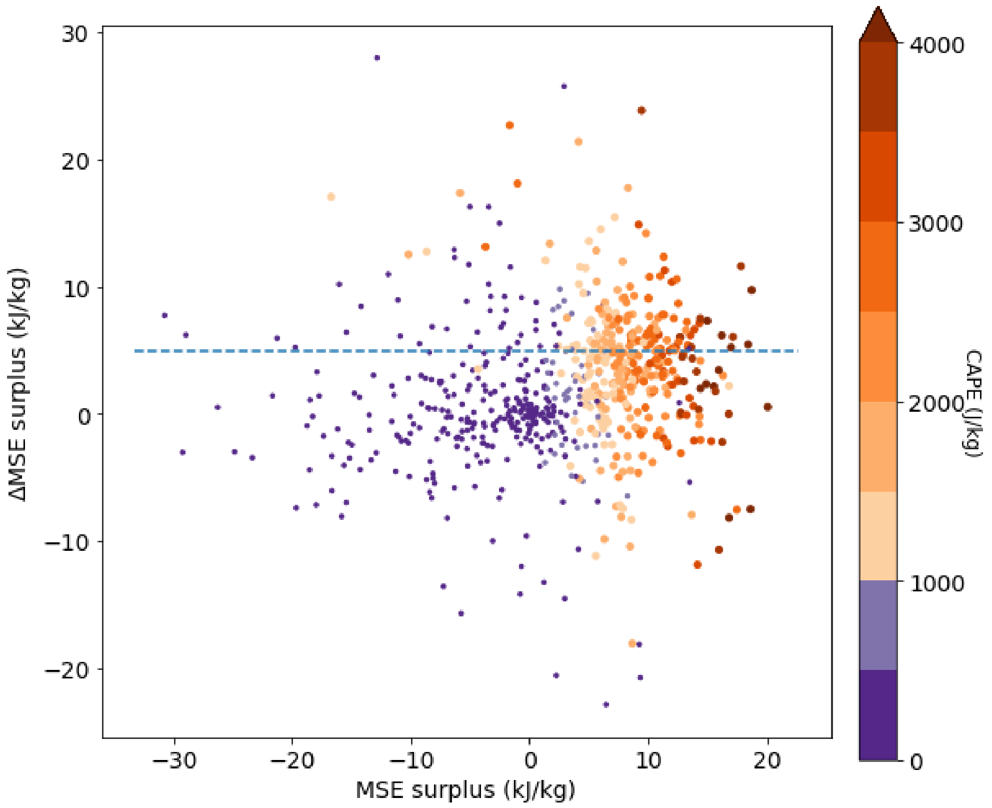


Figure S5k: Scatterplot of MSE surplus change against MSE surplus in current climate, color-coded by CAPE. For clarity, we show one in every 1000 points for CAPE < 1000 J/kg, and one in every 100 for CAPE $\geq$ 1000 J/kg. The dashed line marks the mean MSE surplus change of 4.9 kJ/kg derived from the high CAPE subset as described above. For this subset, MSE surplus changes appear uncorrelated with initial conditions.

## S5.4 Main text Figure 4

This section shows evaluations of how well the four synthetic CAPE distributions considered here match PGW model output. Figure S5l shows CAPE-MSE joint distributions and Table S5e their fitted slopes, and Figure S5m shows CAPE contours in T–H space. In both metrics, the *lapse rate adjustment* outperform other synthetics.

| | PGW | C–C | Constant offset | Lapse rate adj. |
|---|---|---|---|---|
| slope | 0.239 | 0.271 | 0.240 | 0.236 |
| x-intercept (kJ/kg) | 346.2 | 350.4 | 343.8 | 345.8 |

Table S5e: Fitted slopes and intercepts of the future CAPE-MSE framework as in main text Figure 4. *C–C* scaling produces too small a slope and *constant offset* too small an intercept. *Lapse rate adjustment* perform well at both.

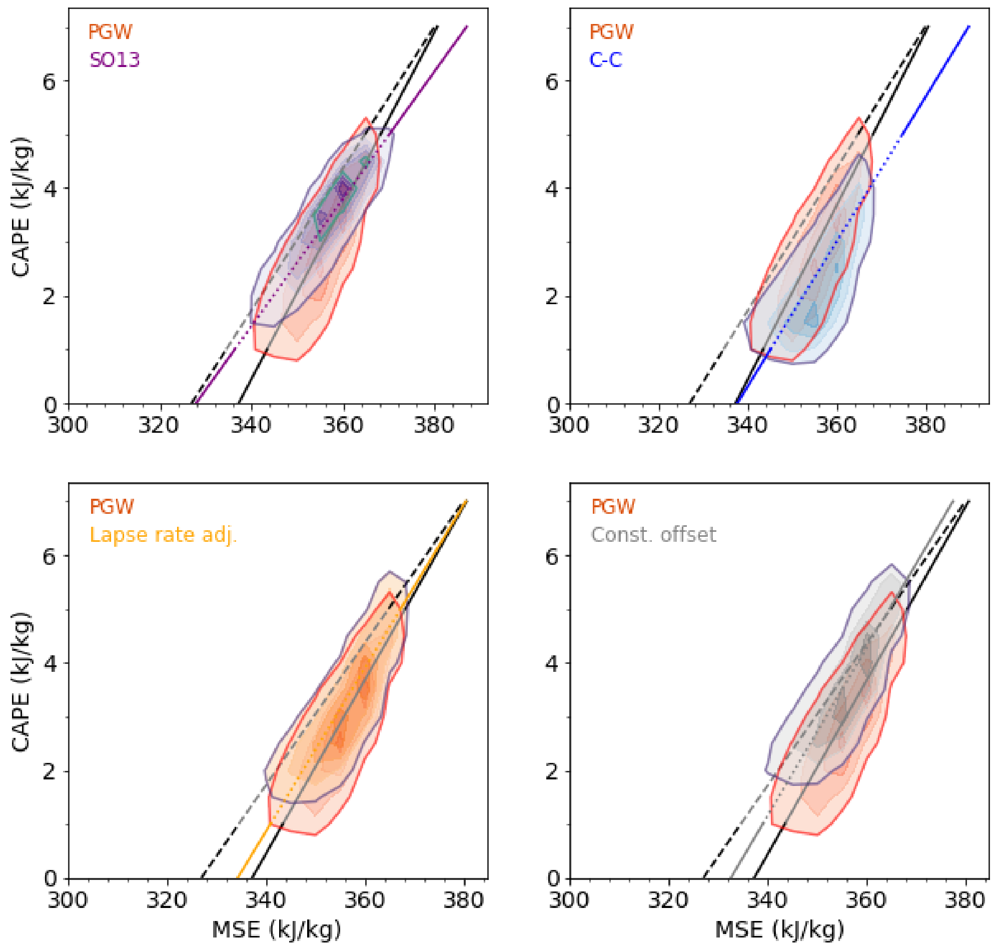


Figure S5l: As in left panel of main text Figure 3, CAPE-MSE density plots for the four synthetic future distributions, separately color-coded. For comparison, model PGW output is shown in red in each panel. Color shading is incremented by 1.5%. Lines show orthogonal distance regressions for CTRL (dashed black), PGW (solid black), and the synthetic (solid colored). *Lapse rate adjustment* visibly outperform other options, though it has problems in the low-CAPE part of the distribution.

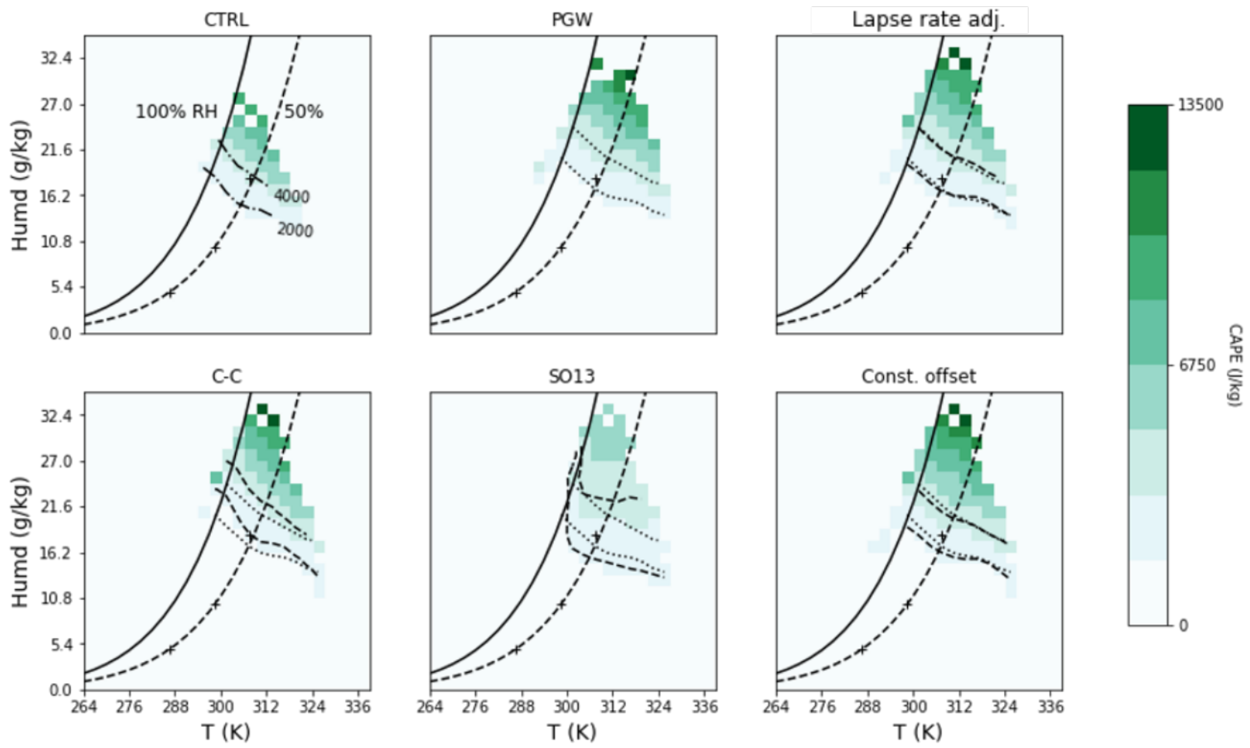


Figure S5m: Mean CAPE in T-H space for CTRL, PGW model output and the different synthetics. Mean CAPE contours at 2000 and 4000 J/kg in each synthetic profile are plotted as dashed lines. PGW contours are plotted as dotted lines, and are repeated in every synthetic plot for comparison. *Lapse rate adjustment* again visibly outperform other options in these high-CAPE conditions.

# S6 Alternative versions of synthetics

## S6.1 SO13 compared to itself vs. to CTRL

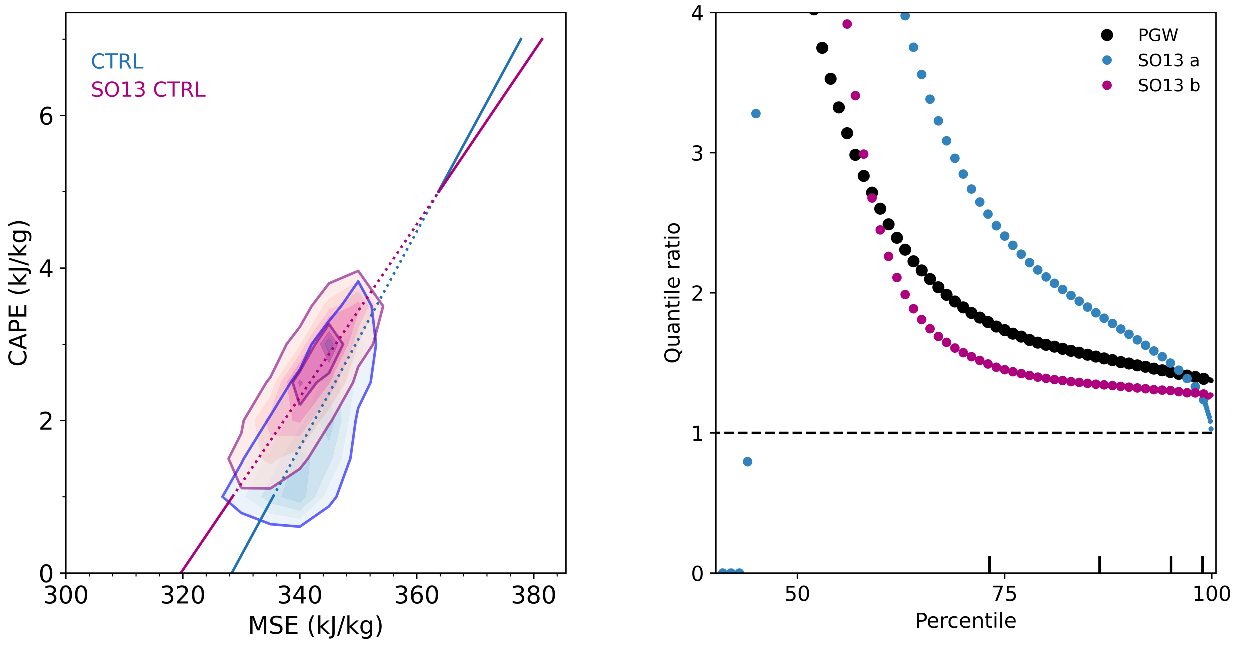


Figure S6a: *Left*: Comparison of CAPE distributions in present-day model output (CTRL) and under the zero-buoyancy model with CTRL surface conditions ($SO13_{CTRL}$). The $SO13_{CTRL}$ CAPE values are too high, and the slope of the CAPE-MSE relationship is too small. *Right*: quantile ratio plots of the future *SO13* synthetic against two present-day distributions: the actual CTRL output ("SO13 a") and the $SO13_{\mathrm{CTRL}}$ prediction ("SO13 b"). See section S4.1 for details on the zero-buoyancy model. We use entrainment rate = 0.62 in both present-day and future versions. Comparing *SO13* to CTRL would imply too-large future CAPE changes, but comparing to $SO13_{CTRL}$, as in the main text, implies too-small changes.

## S6.2 Effect of fixed versus adjusted RH on synthetic transformations

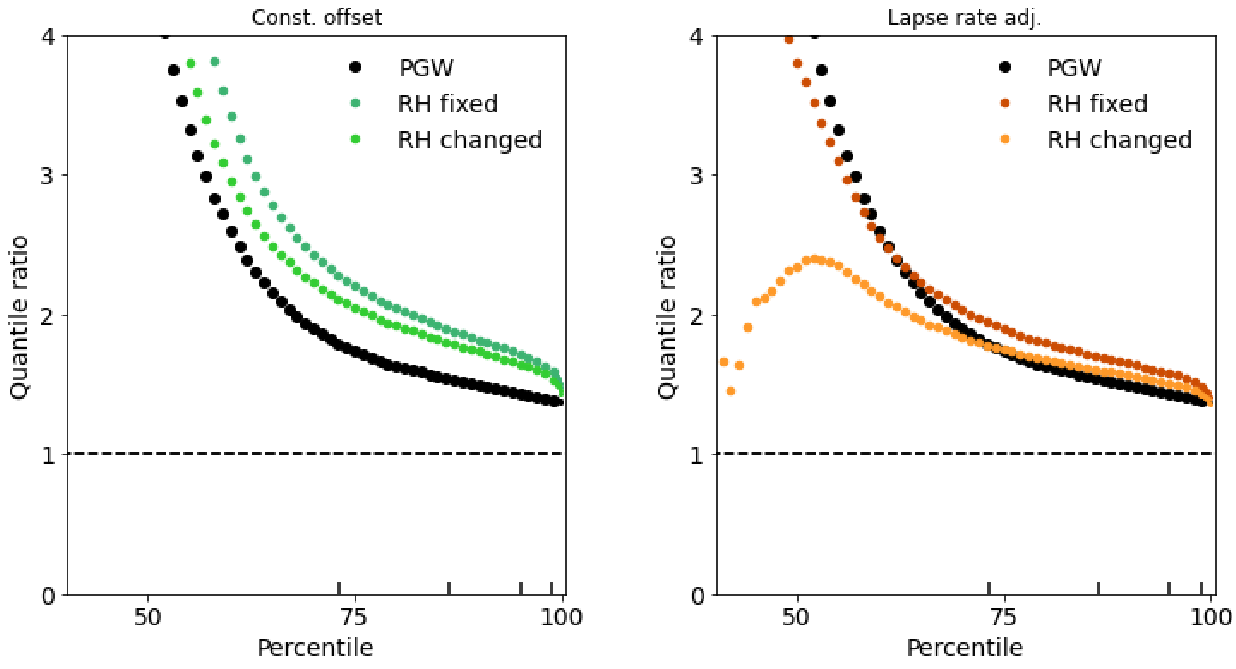


Figure S6b: Quantile ratio plots of PGW and synthetic distributions assuming constant surface RH or a uniform reduction by ∼1%. (Left) For *constant offset*, mean fractional changes are 1.92 with fixed RH and 1.81 with the reduction. Values are derived from average of quantile ratios for ≥ 73rd percentile. (Right) For *lapse rate adjustment*, changes are 1.71 and 1.61. In both cases, the surface RH reduction lowers future CAPE changes by about 6%.

## S7 Latitudinal dependence of changes

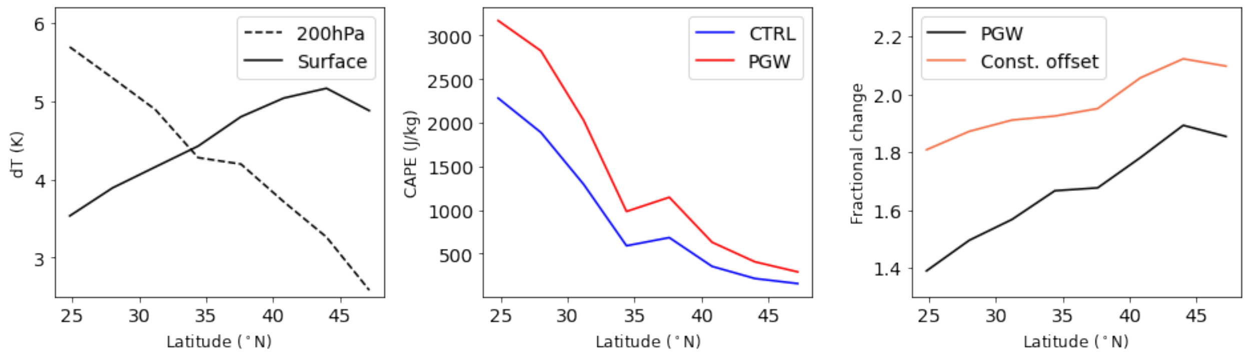


Figure S7a: Latitudinal dependence of changes in temperature and CAPE in model CTRL and PGW runs, for all profiles in the dataset. At lower latitudes, where mean CAPE is higher, future lapse rate changes are positive (surface warms less than upper troposphere), while at higher latitudes the opposite occurs. Fractional CAPE changes across the entire dataset are indeed larger at higher latitudes, but note that they remain smaller than in the *constant offset* case, because mean CAPE changes are still driven by those in the high tail.

## References


Vince Agard and Kerry Emanuel. Clausius–Clapeyron scaling of peak CAPE in continental convective storm environments. *Journal of the Atmospheric Sciences*, 74(9):3043–3054, 2017. ISSN 0022-4928, 1520-0469. doi: 10.1175/JAS-D-16-0352.1.

Kerry Emanuel and Marja Bister. Moist convective velocity and buoyancy scales. *J. Atmos. Sci.*, 53(22):3276–3285, 1996. ISSN 0022-4928. doi: 10.1175/1520-0469(1996)053<3276:MCVABS>2.0.CO;2.

A. Gettelman, D. J. Seidel, M. C. Wheeler, and R. J. Ross. Multidecadal trends in tropical Convective Available Potential Energy. *Journal of Geophysical Research: Atmospheres*, 107:ACL 17–1–ACL 17–8, 2002. ISSN 01480227. doi: 10.1029/2001JD001082.

Stephen A. Klein. Comments on "Moist Convective Velocity and Buoyancy Scales". *Journal of the Atmospheric Sciences*, 54(23):2775–2777, 12 1997. ISSN 0022-4928. doi: 10.1175/1520-0469(1997)054<2775:COMCVA>2.0.CO;2.

Funing Li and Daniel R. Chavas. Midlatitude continental CAPE is predictable from large-scale environmental parameters. *Geophysical Research Letters*, 48(8):e2020GL091799, 2021. ISSN 1944-8007. doi: 10.1029/2020GL091799.

P. Murugavel, S. D. Pawar, and V. Gopalakrishnan. Trends of convective available potential energy over the indian region and its effect on rainfall. *International Journal of Climatology*, 32(9):1362–1372, 2012. doi: 10.1002/joc.2359.

Olivier Pauluis and Isaac M. Held. Entropy budget of an atmosphere in radiative–convective equilibrium. part i: Maximum work and frictional dissipation. *Journal of the Atmospheric Sciences*, 59(2):125–139, 2002. ISSN 0022-4928, 1520-0469. doi: 10.1175/1520-0469(2002)059<0125:EBOAAI>2.0.CO;2.

Kathrin Riemann-Campe, Klaus Fraedrich, and Frank Lunkeit. Global climatology of convective available potential energy (CAPE) and convective inhibition (CIN) in ERA-40 reanalysis. *Atmospheric Research*, 93(1):534–545, 2009. ISSN 01698095. doi: 10.1016/j.atmosres.2008.09.037.

David M. Romps. The dry-entropy budget of a moist atmosphere. *Journal of Atmospheric Sciences*, 65(12):3779–3799, 2008. ISSN 0022-4928, 1520-0469.

Jacob T. Seeley and David M. Romps. Why does tropical Convective available potential energy (cape) increase with warming? *Geophysical Research Letters*, 42(23):10,429–10,437, 2015. doi: 10.1002/2015GL066199.

Martin S. Singh and Paul A. O'Gorman. Influence of entrainment on the thermal stratification in simulations of Radiative-Convective Equilibrium. *Geophysical Research Letters*, 40(16):4398–4403, 2013. ISSN 1944-8007. doi: 10.1002/grl.50796.

Ziwei Wang, James A. Franke, Zhenqi Luo, and Elisabeth J. Moyer. Reanalyses and a high-resolution model fail to capture the "high tail" of CAPE distributions. *Journal of Climate*, 34(21):8699–8715, 2021. ISSN 0894-8755, 1520-0442. doi: 10.1175/JCLI-D-20-0278.1.
